# Supplementary material for: Pion decay constraints on exotic 17 MeV vector bosons
Source: arXiv:2306.15077 source file (2023-09-11)
Supplement: Supplementary file 1 [file appendix_wrapper.tex]

\documentclass[aps,prl,showpacs,letterpaper,twocolumn, floatfix]{revtex4}

\usepackage{graphicx}
\usepackage{bm}
\usepackage{epsf}
\usepackage{rotating}
\usepackage{epsfig,graphics,rotate,color}
\usepackage{wrapfig}
\usepackage{amssymb}
\usepackage{amsmath}
\usepackage{amsfonts}
\usepackage{array,hhline,dcolumn}
\usepackage{gensymb}
\usepackage{placeins}
\usepackage[colorlinks=true,citecolor=blue,linkcolor=blue]{hyperref}
\usepackage{xr}
\usepackage{cleveref}

% this package is just to add random text for this example
\usepackage{blindtext}

\definecolor{nicepurple}{RGB}{102, 2, 60}

\externaldocument{main.tex}

\begin{document}
\input{appendix_text.tex}
\end{document}
